# Supplementary material for: MultiEvoSkill: Structure-Aware Multi-Agent Skill Evolution for Generalizable Skill Artifacts
Source: arXiv:2610.34260 source file (2026-10-25)
Supplement: Supplementary file 1 [file appendix_new.tex]

\section{Relate Work Route}
Existing methods can be grouped by
their update signal and search strategy into trajectory distillation,
execution-feedback refinement, multi-agent evolution,
population-based evolution, and reinforcement-learning-based evolution, 
as summarised in Table~\ref{tab:skill-evolution-taxonomy}.

\begin{table}[h]
\centering
\small
\caption{Major routes for agentic skill evolution.}
\label{tab:skill-evolution-taxonomy}
\begin{tabular}{p{0.29\columnwidth}p{0.62\columnwidth}}
\toprule
\textbf{Route} & \textbf{Representative methods} \\
\midrule
Trajectory distillation
& Trace2Skill~\citep{trace2skill2026},
SkillCAT~\citep{skillcat2026},
SkillEvolver~\citep{skillevolver2026},
Memento-Skills~\citep{zhou2026mementoskills},
WikiSkill~\citep{wikiskill2026} \\

Execution-feedback refinement
& SkillOpt~\citep{skillopt2026},
SkillBoost~\citep{skillboost2026},
SkillGrad~\citep{skillgrad2026},
SkillRevise~\citep{skillrevise2026},
EmbodiSkill~\citep{embodiskill2026} \\

Multi-agent evolution
& CoEvoSkills~\citep{coevoskills2026},
SkillGen~\citep{skillgen2026},
MIND-Skill~\citep{mindskill2026},
SkillHone~\citep{skillhone2026} \\

Population-based evolution
& AgentPSO~\citep{agentpso2026},
MOCHA~\citep{mocha2026},
GEPA~\citep{gepa2025},
EvoSkill~\citep{evoskill2026} \\

Reinforcement-learning-based
& D2Skill~\citep{d2skill2026},
SkillRL~\citep{skillrl2026},
SkillOS~\citep{skillos2026},
Skill1~\citep{skill12026} \\
\bottomrule
\end{tabular}
\end{table}

\section{Implementation Protocol}
\label{app:protocol}
The implementation described here is the graph-only package in the uploaded
\texttt{MultiEvoSkills 2.zip}, rather than the older UnifiedHarness codebase.
The source paper's alternate introduction/method files and outdated experiment
narratives are not part of this revision. Table~\ref{tab:hyperparameters} lists
the main entry-point configuration, which overrides several dataclass defaults.

\begin{table}[h]
\centering\small
\caption{Current domain settings: initialization examples $n_0$, epochs $e$,
batch size $b$, regression base tolerance $\epsilon$, mean-gain threshold $\tau$,
non-decrease fraction $q_0$, and total-selection-size allowance $a$.}
\label{tab:hyperparameters}
\begin{tabular}{@{}lrrrrrrr@{}}
\toprule
Domain & $n_0$ & $e$ & $b$ & $\epsilon$ & $\tau$ & $q_0$ & $a$ \\
\midrule
WikiHow & 40 & 4 & 40 & .03 & .01 & .5 & 0 \\
ToolAlpaca & 40 & 4 & 40 & .03 & .01 & .5 & 0 \\
WebShop & 40 & 4 & 40 & .03 & .01 & .5 & 0 \\
SpreadsheetBench & 40 & 4 & 40 & .10 & .02 & .5 & 1 \\
SearchQA & 40 & 4 & 40 & .02 & .01 & .5 & 1 \\
LiveMath & 35 & 4 & 35 & .02 & .01 & .5 & 1 \\
OfficeQA & 40 & 4 & 40 & .02 & .01 & .5 & 1 \\
\bottomrule
\end{tabular}
\end{table}
Common settings are seed 42, a maximum of two additional batch attempts,
two reflection rounds, two peer edits per proposal revision, one to three
proposal-revision rounds, issue similarity threshold 0.88, debate similarity
threshold 0.95, and up to eight selected issues with two visible evidence rows
each. The embedding endpoint is configured as \texttt{text-embedding-3-small}.
These identifiers describe the code configuration rather than independently
verified provider metadata.

\begin{table}[h]
\centering\small
\caption{Split declarations and primary adapter metrics. A declaration is not
a verification of an absent data file.}
\label{tab:splits}
\begin{tabularx}{\linewidth}{@{}lrrrX@{}}
\toprule
Domain & Train & Selection & Test & Primary metric / qualification \\
\midrule
WikiHow & 157 & 53 & 52 & Node F1; split counts from supplied manuscript. \\
ToolAlpaca & 56 & 19 & 18 & Node F1; counts declared in adapter. \\
WebShop & 80 & 27 & 26 & Node F1; counts declared in adapter. \\
SpreadsheetBench & 80 & 40 & 280 & Hard instance accuracy; counts from manuscript/protocol. \\
SearchQA & 400 & variable & 1400 & Token F1; manuscript says 40 of 200, but entry point loads the complete validation file. \\
LiveMath & 35 & 17 & 125 & Answer accuracy; train/selection counts asserted by sandbox preparation. \\
OfficeQA & 50 & 24 & 172 & Normalized EM; counts asserted by adapter. \\
\bottomrule
\end{tabularx}
\end{table}
The uploaded package does not include the full split files or result manifests.
The three workflow-planning adapters report node recovery, not successful tool
execution. SpreadsheetBench uses a bounded ReAct interaction with a workbook
scorer; OfficeQA uses read-only local document tools. These are different
execution settings and should not be collapsed into a single environment-success
interpretation.

\section{Algorithmic Detail}
\label{app:algorithm}
\begin{enumerate}[leftmargin=*,itemsep=2pt]
\item Initialize or import $G_0$; measure its selection scores using fixed
executor shards. Construct the seeded training schedule.
\item For each scheduled batch, reset transient experience lists and retain the
current persistent parent. Execute the batch once per attempt under fixed item
ownership, optionally appending the transient lists to the executor document.
\item Reflect on each trajectory with all models, revise each analysis with peer
feedback, consolidate within trajectories, and merge across trajectories.
Retrieve relevant historical proposals and build the compact issue payload.
\item Generate issue-specific edits; run bounded revisions against the same
parent. Mechanically apply candidates, but do not measure individual candidate
reward. Keep the full final applicable pool.
\item Build operation interaction regions; process regions by topological level
and degree priority. Keep conflict-free regions and adjudicate conflict regions
with closed-set operation selection. Validate every response and the final
ordered composition.
\item Evaluate the realized candidate on selection shards; request topology
review when enabled; apply the active gate. On acceptance, checkpoint the
candidate and reuse its selection scores as the new parent scores.
\item On a handled pre-gate failure or rejection, accumulate up to five failure
lessons and five success experiences and retry within the same batch budget.
After acceptance or exhaustion, clear transient experience and advance the
schedule. Unhandled infrastructure exceptions can terminate the run.
\item Freeze the last accepted graph and then load the test split. Evaluate the
initial and final frozen artifacts with the configured target; reuse the initial
result when the two fingerprints are identical.
\end{enumerate}

\paragraph{Mechanical validity versus semantic claims.}
The parser and merged-graph validator enforce structural checks, whereas
\texttt{apply\_edit} itself performs mutation on a copy and does not call the
complete validator. A returned \texttt{Skill} object is consequently not a
certificate that a proposal is a valid graph. Similarly, prompt instructions
against changing output protocols or copying reference content do not constitute
an exhaustive semantic verifier. Claims in the main text distinguish these
boundaries deliberately.

\paragraph{Failure handling.}
A malformed regional decision has one schema/ID repair opportunity. A failed
regional merge in the graph-LLM path yields no candidate, rather than returning
a guaranteed deterministic subset. An inconclusive topology jury is different:
it yields an inapplicable topology predicate and can therefore coexist with an
accepted behavioral gate. These failure policies must be reported separately.

\section{Graph--Document Example}
\label{app:mapping}
The formula/value branch in Table~\ref{tab:graph-document} is a four-node,
four-edge subgraph of the existing 18-node spreadsheet example. The topology
contains $7\to8$, $7\to9$, $8\to10$, and $9\to10$, with true/false labels on the
first two edges. The document renders a conditional choice followed by a shared
continuation, not sequential execution of both alternatives. A node's label
carries its action and local restrictions; an edge's note supplies a branch or
ordering explanation. Multiple nodes and edges can therefore map to one
paragraph, while one node may be mentioned by several relational sentences.

The example's later correction step $17\to18$ proceeds to final confirmation;
it is not a loop back to the earlier full validation steps. Graphs that require
an explicit retry can use a labeled loop back-edge to a decision guard, but the
renderer only describes that control flow to the LLM. It does not implement a
separate loop scheduler.

\section{Prompt Responsibilities}
\label{app:prompts}
The following summarizes the current prompt contracts rather than presenting
truncated strings as exact prompts. The source modules are the authoritative
prompt definitions.
\begin{description}[style=nextline]
\item[Initializer.]
Infer a reusable policy from task inputs, exclude reference answers and immutable
output/tool protocol, and return nodes and typed edges in the required JSON
schema. Decision labels and guarded loop annotations carry control information.
\item[Reflector.]
Diagnose only trajectory-supported failures, separate reusable rules from
sample-local evidence, identify graph locations, and record successful behaviors
with applicability conditions. Revisions explain changes relative to the
previous analysis. Reference redaction and location normalization are additional
implementation safeguards.
\item[Proposer.]
Return issue-targeted bounded edits with evidence IDs, expected effects, and
risks. Avoid sample-specific instructions and changes to the harness contract.
The same proposal prompt supports initial generation, peer revision, and an
initial parsing/application-error repair.
\item[Regional merger.]
Candidate evidence evaluation is explicitly described as disabled. Select or
drop only current-region IDs, preserve detected dependencies, avoid conflicting
pairs, and explain drops. Nearby and prior-region operations provide context
without selection authority. JSON repair does not authorize rewriting operations.
\item[Topology jury.]
Review dependencies against node meanings conservatively. Treat explicit
missing, contradictory, or unsupported dependencies as hard issues and mere
redundancy/ambiguity as warnings. A review is advisory until the configured
confidence and vote rules are met.
\end{description}

%\section{Unresolved Result Provenance}
%\label{app:unresolved-results}
%The supplied leave-one-out table contains the entries below. We retain its raw labels and numerical scale because the source does not map $\delta_i$ to named model exclusions or identify a verifiable run/split/metric record. No mapping or rescaling is inferred.
%\begin{table}[h]
%\centering\small
%\caption{Unresolved partial leave-one-out entries preserved verbatim.}
%\begin{tabular}{@{}lrr@{}}
%\toprule
%Source label & WikiHow & SearchQA \\
%\midrule
%w/o $\delta_1$ & 0.4373 & 0.9467 \\
%w/o $\delta_2$ & 0.4553 & 0.9217 \\
%\bottomrule
%\end{tabular}
%\end{table}
%Older prose in the manuscript additionally reports a WikiHow progression, replay-based debate diagnostics, a cost multiplier, and byte-equivalence tests. Those records refer to different configurations and are not accompanied by current run evidence. They have not been promoted into results for the present implementation. The revision audit preserves their removal rationale.
